# Supplementary material for: Performance Characterization of Expert Router for Scalable LLM Inference
Source: arXiv:2404.15153 source file (2024-10-08)
Supplement: Supplementary file 1 [file Appendix_A.tex]

\section{Appendix A}
\label{sec:methods}

\begin{figure*}[ht!]
  \centering
  
  % First row for TP=4
  \rule[0.5ex]{0.3\textwidth}{0.4pt}
  \vspace*{3pt}
  \textbf{TP 4}
  \vspace*{3pt}
  \rule[0.5ex]{0.3\textwidth}{0.4pt}
  \vspace{3pt} % Reduced space between title and images
  
  \begin{subfigure}[t]{0.3\textwidth}
    \centering
    \includegraphics[height=4.5 cm]{02_Hyperparameter_Images_FP16/heatmap_Total Time_TP4_init.pdf}
    \caption*{FP16}
    \label{fig:tp4-fp16}
  \end{subfigure}
  \hspace{0.5em}
  \begin{subfigure}[t]{0.3\textwidth}
    \centering
    \includegraphics[height=4.5 cm]{03_Hyperparameter_Images_INT8/heatmap_Total Time_TP4_init.pdf}
    \caption*{INT8}
    \label{fig:tp4-int8}
  \end{subfigure}
  \hspace{0.5em}
  \begin{subfigure}[t]{0.3\textwidth}
    \centering
    \includegraphics[height=4.5 cm]{04_Hyperparameter_Images_INT4/heatmap_Total Time_TP4_init.pdf}
    \caption*{INT4}
    \label{fig:tp4-int4}
  \end{subfigure}

  \vspace{8pt} % Space between rows

  % Second row for TP=8
  \rule[0.5ex]{0.3\textwidth}{0.4pt}
  \vspace*{3pt}
  \textbf{TP 8}
  \vspace*{3pt}
  \rule[0.5ex]{0.3\textwidth}{0.4pt}
  \vspace{3pt} % Reduced space between title and images
  
  \begin{subfigure}[t]{0.3\textwidth}
    \centering
    \includegraphics[height=4.5 cm]{02_Hyperparameter_Images_FP16/heatmap_Total Time_TP8_init.pdf}
    \caption*{FP16}
    \label{fig:tp8-fp16}
  \end{subfigure}
  \hspace{0.5em}
  \begin{subfigure}[t]{0.3\textwidth}
    \centering
    \includegraphics[height=4.5 cm]{03_Hyperparameter_Images_INT8/heatmap_Total Time_TP8_init.pdf}
    \caption*{INT8}
    \label{fig:tp8-int8}
  \end{subfigure}
  \hspace{0.5em}
  \begin{subfigure}[t]{0.3\textwidth}
    \centering
    \includegraphics[height=4.5 cm]{04_Hyperparameter_Images_INT4/heatmap_Total Time_TP8_init.pdf}
    \caption*{INT4}
    \label{fig:tp8-int4}
  \end{subfigure}

  \caption{\textbf{Throughput data for different Model configurations based on tensor parallelism levels TP 4 and TP 8.} }
  \label{fig:all_images}
\end{figure*}
